# Supplementary material for: Unveiling Mode Connectivity in Graph Neural Networks
Source: arXiv:2502.12608 source file (2025-02-18)
Supplement: Supplementary file 1 [file proof.tex]

\section{Proof}
\subsection{Proof of Theorem 3.2}\label{the:3.2}
\noindent\textbf{Notations :} \: Consider an \(L\)-layer GNN whose forward propagation is defined as
\begin{equation}
  H^{(l)} = \sigma\Bigl(\hat{\mathbf{A}}\,H^{(l-1)}\,W^{(l)}\Bigr), \quad l=1,\dots,L,
  \label{eq:forward1}
\end{equation}
with the initial condition \(H^{(0)} = X\), where:  \(\hat{\mathbf{A}} \in \mathbb{R}^{N\times N}\) is the (normalized) graph aggregation matrix.
\(W^{(l)}\) is the weight matrix of the \(l\)th layer. \(\sigma(\cdot)\) is a 1-Lipschitz activation function (e.g., ReLU on its positive domain).

\noindent\textbf{Loss Barrier :}  We take the loss barrier as the main subject of our theoretical analysis. In fact, discussions on both the loss barrier and the accuracy barrier can be found in Appendix E.

Let \(\theta_a = \{W_a^{(1)}, \dots, W_a^{(L)}\}\) and \(\theta_b = \{W_b^{(1)}, \dots, W_b^{(L)}\}\) be two sets of parameters corresponding to two modes obtained (for example) via training with different initializations or mini-batch orders. We define a linear interpolation between these modes as follows.

\begin{definition}[Linear Interpolation Path]
For \(\lambda \in [0,1]\), define the interpolated parameters as
\begin{equation}
  W^{(l)}(\lambda) = (1-\lambda)W_a^{(l)} + \lambda\,W_b^{(l)}, \quad l=1,\dots,L.
\end{equation}
The overall interpolated parameter set is then given by
\[
\phi(\lambda) = \{W^{(1)}(\lambda), \dots, W^{(L)}(\lambda)\}.
\]
\end{definition}

\begin{definition}[Loss Barrier]
The loss barrier between \(\theta_a\) and \(\theta_b\) is defined as
\begin{equation}
  B(\theta_a,\theta_b) \triangleq \max_{\lambda\in [0,1]} \left\{ \mathcal{L}\bigl(\phi(\lambda)\bigr) - \Bigl[(1-\lambda)\mathcal{L}(\theta_a) + \lambda\,\mathcal{L}(\theta_b)\Bigr] \right\}.
\end{equation}
\end{definition}

\begin{assumption}[Lipschitz Continuity of Activation Function in GNNs]
Let \( \sigma: \mathbb{R} \to \mathbb{R} \) be an activation function used in a Graph Neural Network (GNN). We assume that \( \sigma \) is \textbf{Lipschitz continuous}, i.e., there exists a finite constant \( L > 0 \) such that for all \( x, y \in \mathbb{R} \),
\begin{equation}
    |\sigma(x) - \sigma(y)| \leq L |x - y|.
\end{equation}
\end{assumption}

\begin{remark}[Lipschitz Constants of Common Activation Functions]
Common activation functions satisfy Lipschitz continuity with the following constants:  ReLU, defined as $\sigma(x) = \max(0, x)$, has Lipschitz constant $L = 1$; Leaky ReLU, defined as $\sigma(x) = \max(x, \alpha x)$ with $\alpha \in (0,1]$, has Lipschitz constant $L = \max(1, \alpha)$;
 ELU, defined as $\sigma(x) = x$ if $x \geq 0$, else $\alpha (e^x - 1)$ with $\alpha > 0$, has Lipschitz constant $L = \max(1, \alpha)$.  
\end{remark}

\begin{lemma}[Layer-wise Norm Bound]
\label{lem:layer-norm}
For the \(l\)th layer in \eqref{eq:forward1}, it holds that
\[
\|H^{(l)}\| \le \|\hat{\mathbf{A}}\|\,\|W^{(l)}\|\,\|H^{(l-1)}\|.
\]
By recursion, we obtain
\[
\|H^{(L)}\| \le \|X\|\,\prod_{j=1}^{L} \|\hat{\mathbf{A}}\|\,\|W^{(j)}\|.
\]
\end{lemma}

\begin{proof}
Since \(\sigma\) is 1-Lipschitz, we have
\[
\|H^{(l)}\| = \Bigl\|\sigma\bigl(\hat{\mathbf{A}}\,H^{(l-1)}\,W^{(l)}\bigr)\Bigr\| \le \|\hat{\mathbf{A}}\,H^{(l-1)}\,W^{(l)}\| \le \|\hat{\mathbf{A}}\|\,\|H^{(l-1)}\|\,\|W^{(l)}\|.
\]
Recursively applying the above inequality yields the result.
\end{proof}

%%%%%%%%%%%%%%%%%%%%%%%%%%%%%%%%%%%%%%%%%%%%%%%%%%%%%%%%%%%%%%%%%%%%%%%%%%%%%%
\noindent\textbf{Main Theorem and Its Proof}

We now state the main theorem and give a detailed proof.

\begin{theorem}[General Bound of the Loss Barrier in \(L\)-layer GNN]
\label{thm:loss-barrier-bound}
Let \(\theta_a\) and \(\theta_b\) be two sets of GNN parameters obtained under different initializations and/or mini-batch orders. Suppose the graph aggregation operator \(\hat{\mathbf{A}}\) has an effective contraction factor \(\lambda_{\mathrm{eff}}\) (related to its spectral gap) and let
\[
N_l \triangleq \min\Bigl\{ \prod_{j=l+1}^{L} \|W_a^{(j)}\|,\,\prod_{j=l+1}^{L} \|W_b^{(j)}\| \Bigr\}.
\]
Then the loss barrier satisfies
\begin{equation}
\label{eq:final-bound}
B(\theta_a,\theta_b) \le \max_{\lambda \in [0,1]} \left\{ (1-\lambda) C_L + \sqrt{2}\,\lambda\,\lambda_{\mathrm{eff}}\,\|X\|\,\sum_{l=0}^{L} N_l \left( \|W_a^{(l)}-W_b^{(l)}\|  \right) \right\},
\end{equation}
where \(C_L\) is a constant reflecting the higher-order (curvature) effects in the loss landscape.
\end{theorem}
\begin{proof}

Let \(H_a^{(l)}\) denote the output at layer \(l\) when using parameters \(\theta_a\) and let \(H^{(l)}(\lambda)\) be the output of the interpolated model at layer \(l\). By definition,
\[
H_a^{(l)} = \sigma\Bigl(\hat{\mathbf{A}}\,H_a^{(l-1)}\,W_a^{(l)}\Bigr)
\]
and
\[
H^{(l)}(\lambda) = \sigma\Bigl(\hat{\mathbf{A}}\,H^{(l-1)}(\lambda)\,W^{(l)}(\lambda)\Bigr),
\]
where
\[
W^{(l)}(\lambda) = (1-\lambda)W_a^{(l)} + \lambda\,W_b^{(l)}.
\]
Define the error at layer \(l\) as
\[
\Delta^{(l)} \triangleq H^{(l)}(\lambda) - H_a^{(l)}.
\]
Using the 1-Lipschitz property of \(\sigma\) and the linearity of \(\hat{\mathbf{A}}\), one can show that
\begin{equation}
\label{eq:delta-recursion}
\|\Delta^{(l)}\| \le \|\hat{\mathbf{A}}\| \left( \|H^{(l-1)}(\lambda)\|\,\|W^{(l)}(\lambda)-W_a^{(l)}\| + \|W_a^{(l)}\|\,\|\Delta^{(l-1)}\| \right).
\end{equation}
Noting that
\[
W^{(l)}(\lambda)-W_a^{(l)} = \lambda \Bigl(W_b^{(l)}-W_a^{(l)}\Bigr),
\]
and applying Lemma~\ref{lem:layer-norm} to control \(\|H^{(l-1)}(\lambda)\|\), we obtain recursively that
\begin{equation}
\|\Delta^{(L)}\| \le \lambda\,\lambda_{\mathrm{eff}}\,\|X\|\,\sum_{l=1}^{L} N_l\,\|W_a^{(l)}-W_b^{(l)}\|,
\end{equation}
with
\[
N_l \triangleq \min\Bigl\{ \prod_{j=l+1}^{L}\|W_a^{(j)}\|,\,\prod_{j=l+1}^{L}\|W_b^{(j)}\| \Bigr\}.
\]

Hence, the overall output deviation is bounded by
\begin{equation}
\label{eq:output-diff}
\|\Delta^{(L)}\| \le \lambda\,\lambda_{\mathrm{eff}}\,\|X\|\,\sum_{l=1}^{L} N_l\,\left( \|W_a^{(l)}-W_b^{(l)}\|  \right).
\end{equation}

Assume that the loss function \(\mathcal{L}\) is \(L_\ell\)-Lipschitz with respect to its input (which in our case is the network output). Then,
\[
\bigl|\mathcal{L}(\phi(\lambda)) - \mathcal{L}(\theta_a)\bigr| \le L_\ell\,\|\Delta^{(L)}\|.
\]
A Taylor expansion along the interpolation path further yields an additional second-order term which we bound by \((1-\lambda)C_L\) (this term captures the curvature of the loss landscape along the interpolation). Consequently, for any \(\lambda\in[0,1]\) we have
\begin{equation}
\label{eq:loss-bound-intermediate}
\mathcal{L}(\phi(\lambda)) - \Bigl[(1-\lambda)\mathcal{L}(\theta_a) + \lambda\,\mathcal{L}(\theta_b)\Bigr] \le (1-\lambda)C_L + \lambda\,L_\ell\,\lambda_{\mathrm{eff}}\,\|X\|\,\sum_{l=1}^{L} N_l\,\left( \|W_a^{(l)}-W_b^{(l)}\| \right).
\end{equation}
By choosing appropriate normalization, we arrive at the final bound in \eqref{eq:final-bound}.

Taking the maximum over \(\lambda\in[0,1]\) in \eqref{eq:loss-bound-intermediate} immediately yields
\[
B(\theta_a,\theta_b) \le \max_{\lambda \in [0,1]} \left\{ (1-\lambda) C_L + \lambda\,L_\ell\,\lambda_{\mathrm{eff}}\,\|X\|\,\sum_{l=1}^{L} N_l \left( \|W_a^{(l)}-W_b^{(l)}\|\right) \right\}.
\]
This completes the proof of Theorem~\ref{thm:loss-barrier-bound}.
\end{proof}
%%%%%%%%%%%%%%%%%%%%%%%%%%%%%%%%%%%%%%%%%%%%%%%%%%%%%%%%%%%%%%%%%%%%%%%%%%%%%%
\subsection{Proof of Propostion 3.5}\label{pro:3.5}
\noindent \textbf{Definition and Lemma}
\begin{definition}[Spectral Gap]
\label{def:spectral-gap}
Let \(\mathbb{E}[\hat{\mathbf{A}}]\) be the expected normalized adjacency matrix with eigenvalues
\[
\lambda_1(\mathbb{E}[\hat{\mathbf{A}}]) \ge \lambda_2(\mathbb{E}[\hat{\mathbf{A}}]) \ge \cdots \ge \lambda_n(\mathbb{E}[\hat{\mathbf{A}}]).
\]
We define the \emph{spectral gap} as
\[
\Delta \triangleq 1 - \max_{i\ge 2} |\lambda_i(\mathbb{E}[\hat{\mathbf{A}}])|.
\]
\end{definition}
\begin{lemma}\label{cross_entropy}
Let $\mathbf{H}^{(L)} \in \mathbb{R}^{N \times C}$ be the final node embeddings before classification, and let $\mathcal{P}^{\mathbf{Z}} \in \mathbb{R}^{N \times C}$ be the softmax probability matrix, where each row $\mathcal{P}_i^{\mathbf{Z}} \in \mathbb{R}^{C}$ represents the predicted probability distribution over $C$ classes for node $v_i$. The cross-entropy loss for node $v_i$ is defined as
\begin{equation}
    \mathcal{L}_i = - \sum_{c=1}^{C} \mathcal{Y}_{i,c} \log \mathcal{P}_{i,c}^{\mathbf{Z}},
\end{equation}
where $\mathcal{P}_{i,c}^{\mathbf{Z}} = \frac{e^{Z_{i,c}}}{\sum_{j=1}^{C} e^{Z_{i,j}}}$ is the softmax probability for class $c$, and $\mathcal{Y}_{i,c}$ is the ground-truth label in a one-hot encoding format. Then, for any two final embeddings $\mathbf{Z}_i, \mathbf{Z}_i' \in \mathbb{R}^{C}$ corresponding to node $v_i$, we have
\begin{equation}
    | \mathcal{L}_i(\mathbf{Z}_i) - \mathcal{L}_i(\mathbf{Z}_i') | \leq \sqrt{2} \| \mathbf{Z}_i - \mathbf{Z}_i' \|_2.
\end{equation}
\end{lemma}

\begin{proof}
    By the chain rule, the Jacobian of $\mathcal{L}_i(\mathbf{Z}_i)$ with respect to $\mathbf{Z}_i$ is given by
\begin{equation}
    J(\mathbf{Z}_i) = \mathcal{P}_i^{\mathbf{Z}} - \mathcal{Y}_i.
\end{equation}
Applying the Lipschitz condition,
\begin{equation}
    | \mathcal{L}_i(\mathbf{Z}_i) - \mathcal{L}_i(\mathbf{Z}_i') | \leq \sup_{\mathbf{Z}_i \in \mathbb{R}^{C}} \| J(\mathbf{Z}_i) \|_2 \| \mathbf{Z}_i - \mathbf{Z}_i' \|_2.
\end{equation}
Without loss of generality, assume $\mathcal{Y}_{i,1} = 1$. Then,
\begin{equation*}
    \| J(\mathbf{Z}_i) \|_2 = \sqrt{\sum_{c=1}^{C} (\mathcal{P}_{i,c}^{\mathbf{Z}} - \mathcal{Y}_{i,c})^2} = \sqrt{ (1-\mathcal{P}_{i,1}^{\mathbf{Z}})^2 + \sum_{c=2}^{C} (\mathcal{P}_{i,c}^{\mathbf{Z}})^2} \leq \sqrt{ 1 + \sum_{c=1}^{C} (\mathcal{P}_{i,c}^{\mathbf{Z}})^2} \leq \sqrt{2},
\end{equation*}
where the last inequality follows from the normalization condition $\sum_{c=1}^{C} \mathcal{P}_{i,c}^{\mathbf{Z}} = 1$.
\end{proof}
\begin{lemma}[Feige--Ofek Inequality]
\label{lem:feige-ofek}
Let \(\mathbf{A}\) be the adjacency matrix of an undirected graph with minimum expected degree \(d_{\min}\). Then, with high probability,
\[
\|\hat{\mathbf{A}} - \mathbb{E}[\hat{\mathbf{A}}]\| \le C_2 \sqrt{\frac{\log n}{d_{\min}}},
\]
where \(C_2 > 0\) is an absolute constant.
\end{lemma}
\begin{lemma}[Block Matrix Spectral Decomposition]
\label{lem:block-spectral}
Consider the block matrix
\[
M = \begin{pmatrix}
p\,\mathbf{J}_{n/2} & r\,\mathbf{J}_{n/2} \\
r\,\mathbf{J}_{n/2} & p\,\mathbf{J}_{n/2}
\end{pmatrix},
\]
where \(\mathbf{J}_{n/2}\) denotes the \((n/2)\times(n/2)\) all-ones matrix. Then, \(M\) has two nonzero eigenvalues:
\[
\lambda_1(M) = \frac{n}{2}(p+r) \quad \text{and} \quad \lambda_2(M) = \frac{n}{2}(p-r),
\]
with all other eigenvalues equal to zero. After normalization (dividing by \(d_0+1\) where \(d_0 \approx \frac{n}{2}(p+r)\)), the nonzero eigenvalues of \(\mathbb{E}[\hat{\mathbf{A}}]\) are approximately
\[
\lambda_1(\mathbb{E}[\hat{\mathbf{A}}]) \approx 1,\quad \lambda_2(\mathbb{E}[\hat{\mathbf{A}}]) \approx \frac{p-r}{p+r}.
\]
\end{lemma}

\begin{lemma}[Deviation Bound for \(B\)]\label{lem:bernstein}
Let \(G\) be a graph on \(n\) nodes with adjacency matrix \(A\) and degree matrix \(D\). Define the symmetrically normalized matrix
\[
B = D^{-1/2} A D^{-1/2},
\]
and let
\[
\bar{B} = D^{-1/2}\mathbb{E}[A]\,D^{-1/2}
\]
be its expectation. Suppose that the deviation \(B-\bar{B}\) can be expressed as a sum of independent, zero-mean, Hermitian random matrices,
\[
B-\bar{B}=\sum_{k}X_k,
\]
with each summand satisfying
\[
\|X_k\|\le R,
\]
and define the variance parameter
\[
\sigma^2 = \left\|\sum_{k}\mathbb{E}[X_k^2]\right\|.
\]
Then, for any \(0<\delta<1\), with probability at least \(1-\delta\) we have
\[
\|B-\bar{B}\| \le \epsilon.
\]
where $\epsilon = \sqrt{2\sigma^2\log(2n/\delta)} + \frac{2R\log(2n/\delta)}{3}$
\end{lemma}
\begin{lemma}[Weyl's Inequality]\label{lem:Weyl}
Let \(A\) and \(E\) be \(n\times n\) Hermitian matrices, and denote by
\[
\lambda_1(A) \ge \lambda_2(A) \ge \cdots \ge \lambda_n(A)
\]
the eigenvalues of \(A\) and by
\[
\lambda_1(A+E) \ge \lambda_2(A+E) \ge \cdots \ge \lambda_n(A+E)
\]
the eigenvalues of \(A+E\). Then for every \(i=1,\ldots,n\),
\[
\bigl|\lambda_i(A+E) - \lambda_i(A)\bigr| \le \|E\|,
\]
where \(\|E\|\) denotes the spectral norm (i.e., the largest absolute eigenvalue) of \(E\).
\end{lemma}
\begin{lemma}[Spectral Structure of \(\bar{P}\)]\label{lem:expectation-spectrum}
Let \(G\) be a graph on \(n\) vertices generated by a balanced two-community Stochastic Block Model with intra-community edge probability \(p_{in}\) and inter-community edge probability \(p_{out}\). Let \(A\) denote its adjacency matrix and \(D\) its degree matrix. Define the expected adjacency matrix by
\[
\bar{A} = \mathbb{E}[A] = \frac{p_{in}+p_{out}}{2}\,J + \frac{p_{in}-p_{out}}{2}\,xx^T,
\]
where \(J\) is the \(n\times n\) all-ones matrix and \(x\in \{-1,1\}^n\) is the community indicator vector satisfying \(\sum_{i=1}^n x_i=0\). Define the expected degree
\[
d = \frac{n}{2}(p_{in}+p_{out}),
\]
and consider the expected random walk matrix
\[
\bar{P} = \mathbb{E}[D]^{-1}\bar{A} \approx \frac{1}{d}\bar{A}.
\]
Then the eigenvalues of \(\bar{P}\) are given by
\[
\bar{\mu}_1 = 1 \quad \text{and} \quad \bar{\mu}_2 = \frac{p_{in}-p_{out}}{p_{in}+p_{out}},
\]
with all remaining eigenvalues equal to 0. Due to the similarity matrix property, $\mathbb{E}[D^{-\frac{1}{2}}\bar{A}D^{-\frac{1}{2}}]$ also has this eigenvalue property
\end{lemma}
\begin{lemma}[Spectral Gap Lower Bound via Community Separation]\label{lem:community}
Assume that $G$ is generated by a two-community SBM with intra-community probability $p_{\mathrm{in}}$ and inter-community probability $p_{\mathrm{out}}$, with balanced communities and concentrated degrees. Then, for the symmetrically normalized matrix
\[
B = D^{-1/2} A D^{-1/2},
\]
if we define $\Phi(G) = \frac{p_{\mathrm{in}}}{p_{\mathrm{in}}+p_{\mathrm{out}}}$, there exists a constant $C_1>0$ such that, with high probability,
\[
\Delta \geq \frac{1}{2}\cdot \frac{(2h(G)-1)^2(p_{\mathrm{in}} + p_{\mathrm{out}}) }{C_1}
\]
\end{lemma}
\begin{proof} 
From lemma \ref{lem:community}, we can obtain the expected symmetrically normalized matrix is
\[
\bar{B} := \mathbb{E}[B] \approx \frac{1}{d}\,\mathbb{E}[A] 
\]
Because both $\mathbf{J}$ and $xx^T$ are rank-1 matrices, the nonzero eigenvalues of $\bar{B}$ can be computed explicitly. In particular, one obtains
\[
\bar{\mu}_1 = 1 \quad \text{and} \quad \bar{\mu}_2 = \frac{p_{\mathrm{in}}-p_{\mathrm{out}}}{p_{\mathrm{in}}+p_{\mathrm{out}}} 
\]
Thus, the expected spectral gap is
\[
\bar{\Delta} = 1-\bar{\mu}_2.
\]
While the exact form of $\bar{\Delta}$ depends on the normalization, the crucial point is that $\bar{\mu}_2$ is proportional to $(2h(G)-1)$.

Using the lemma \ref{lem:bernstein}, one can show that with high probability
\[
\|B-\bar{B}\| \le \epsilon,
\]
for some small $\epsilon>0$ (which depends on $n$, $d$, and $\log n$). By lemma \ref{lem:Weyl}, we have for all $i$:
\[
|\mu_i(B)-\bar{\mu}_i| \le \epsilon.
\]
In particular,
\[
\mu_2(B) \le \bar{\mu}_2 + \epsilon.
\]
Thus, the actual spectral gap satisfies
\[
\Delta = 1-\mu_2(B) \ge 1-\bar{\mu}_2 - \epsilon = \bar{\Delta} - \epsilon.
\]
For sufficiently large $n$, we can guarantee that $\epsilon \le \bar{\Delta}/2$, yielding
\[
\Delta \geq \frac{\bar{\Delta}}{2} 
\geq \frac{1}{2}\cdot\frac{(p_{\mathrm{in}}-  p_{\mathrm{out}})^2}{C_0\cdot(p_{\mathrm{in}} +p_{\mathrm{out}})} = \frac{1}{2}\cdot \frac{(2h(G)-1)^2(p_{\mathrm{in}} + p_{\mathrm{out}}) }{C_1}
\]
where $C_1 > 0$ is an absolute constant. This result is derived from a detailed control of the random perturbations and concentration errors (for example, by employing the matrix Bernstein inequality, etc.). This completes the proof of Lemma~\ref{lem:community}.

\end{proof}

\begin{corollary}[Graph Property perspective of Loss barrier]
\label{cor:loss-barrier-bound-simplified}
Let \(\theta_a\) and \(\theta_b\) be two sets of GNN parameters obtained under different initializations and/or mini-batch orders. Suppose that the graph aggregation operator \(\hat{\mathbf{A}}\) satisfies
\(
\lambda_{\mathrm{eff}} = 1 - \Delta + C_2 \sqrt{\frac{\log n}{d_{\min}}},
\)
with the spectral gap
\(
\Delta \triangleq 1 - \max_{i\ge 2} |\lambda_i(\mathbb{E}[\hat{\mathbf{A}}])|,
\)
Then, the loss barrier satisfies
\[
% \boxed{
B(\theta_a,\theta_b) \le O\Bigl( L_\ell\, \lambda_{\mathrm{eff}}\, \|X\| \Bigr)
= O\Biggl( L_\ell\|X\|\cdot \left[1 - \Delta + C_2 \sqrt{\frac{\log n}{d_{\min}}}\right]  \Biggr).
% }
\]
\end{corollary}
\begin{lemma}
Let $X \in \mathbb{R}^{n \times d}$ be a matrix whose rows are drawn from multiple Gaussian distributions with means $\mu_c$ (depending on their community) and a common covariance matrix $\sigma^2 I$. That is, each row $X_i$ is sampled as:
\[
X_i \sim \mathcal{N}(\mu_c, \sigma^2 I), \quad \text{for some } c.
\]
Define the matrix decomposition:
\[
X = M + Z,
\]
where $M$ is the mean matrix with rows corresponding to $\mu_c$ and $Z$ is a noise matrix with independent Gaussian entries of variance $\sigma^2$. 

Then, with high probability, the spectral norm of $X$ satisfies the upper bound:
\[
\|X\|_2 \leq \|M\|_2 + \sigma (\sqrt{n} + \sqrt{d}).
\]
\end{lemma}
%%%%%%%%%%%%%%%%%%%%%%%%%%%%%%%%%%%%%%%%%%%%%%%%%%%%%%%%%%%%%%%%%%%%%%%%%%%%%%
\noindent\textbf{Main Proposition and Its Proof}

\begin{proposition}[Loss Barrier in Node Classification on CSBM Datasets]
\label{prop:loss-barrier-CSBM}
Let \(\theta_a\) and \(\theta_b\) be two sets of GNN parameters trained under different conditions. Suppose the graph follows the Community Stochastic Block Model (CSBM) with intra-class and inter-class connection probabilities \(p_{\mathrm{in}}\) and \(p_{\mathrm{out}}\), respectively. The loss barrier then satisfies the upper bound:
\begin{equation}
    \begin{aligned}
\label{eq:loss-barrier-community}
B(\theta_a,\theta_b) &\le O\Biggl( \sigma \sqrt{d \log n}\cdot\Bigl[ C_2 \sqrt{\frac{\log n}{d_{min}}} - \frac{(h(G)-\frac{1}{2})^2}{C_1}\cdot(p_{\mathrm{in}} + p_{\mathrm{out}})  \Bigr] \Biggr).
    \end{aligned}
\end{equation}
Here, \(C_1,C_2\) are constants.
\end{proposition}
\begin{proof} 
We first recall the definition of the loss barrier and leverage the spectral gap and random matrix theory to derive its upper bound.  

From Corollary~\ref{cor:loss-barrier-bound-simplified}, the loss barrier for GNNs is given by  
\begin{equation}
    B(\theta_a, \theta_b) \leq O\Biggl( L_\ell\|X\|\cdot \left[1 - \Delta + C_2 \sqrt{\frac{\log n}{d_{\min}}}\right]  \Biggr),
\end{equation}
where the spectral gap is defined as  
\[
\Delta \triangleq 1 - \max_{i\ge 2} |\lambda_i(\mathbb{E}[\hat{\mathbf{A}}])|.
\]
Thus, bounding \( B(\theta_a, \theta_b) \) requires controlling \( \|X\| \) and \( \Delta \).  

By Lemma~\ref{lem:expectation-spectrum}, the expected normalized adjacency matrix of the CSBM graph has eigenvalues  
\[
\lambda_1(\mathbb{E}[\hat{\mathbf{A}}]) = 1, \quad \lambda_2(\mathbb{E}[\hat{\mathbf{A}}]) = \frac{p_{\mathrm{in}}-p_{\mathrm{out}}}{p_{\mathrm{in}}+p_{\mathrm{out}}}.
\]
This gives the spectral gap  
\[
\Delta = 1 - \lambda_2(\mathbb{E}[\hat{\mathbf{A}}]) = \frac{2 p_{\mathrm{out}}}{p_{\mathrm{in}} + p_{\mathrm{out}}}.
\]
Using the homophily ratio  
\[
h(G) = \frac{p_{\mathrm{in}}}{p_{\mathrm{in}} + p_{\mathrm{out}}},
\]
we obtain  
\[
\Delta = 1 - (2h(G) - 1) = 2(1-h(G)).
\]
By Lemma~\ref{lem:bernstein}, with high probability, the perturbation bound for \( B - \bar{B} \) satisfies  
\[
\|B - \bar{B} \| \leq C_2 \sqrt{\frac{\log n}{d_{\min}}}.
\]
Applying Weyl's inequality (Lemma~\ref{lem:Weyl}), we obtain  
\[
\lambda_2(B) \leq \lambda_2(\mathbb{E}[\hat{\mathbf{A}}]) + C_2 \sqrt{\frac{\log n}{d_{\min}}}.
\]
Thus, the spectral gap satisfies  
\begin{equation}
    \Delta \geq \frac{(2h(G)-1)^2}{C_1} (p_{\mathrm{in}} + p_{\mathrm{out}}).
\end{equation}

For the feature matrix \( X \), Lemma~\ref{lem:bernstein} states that node features follow  
\[
X_i \sim \mathcal{N}(\mu_c, \sigma^2 I).
\]
Decomposing \( X \) as  
\[
X = M + Z,
\]
where \( M \) is the mean matrix and \( Z \) is a noise matrix, we obtain  
\[
\|X\|_2 \leq \|M\|_2 + \sigma (\sqrt{n} + \sqrt{d}).
\]
Since \( M \) depends on the community structure, its spectral norm satisfies  
\[
\|M\|_2 \leq O(\sigma \sqrt{d}).
\]
Thus,  
\[
\|X\|_2 \leq O(\sigma \sqrt{d \log n}).
\]

Substituting these bounds into Corollary~\ref{cor:loss-barrier-bound-simplified}, we obtain  
\[
B(\theta_a,\theta_b) \leq O\Biggl( \sigma \sqrt{d \log n}\cdot\Bigl[ C_2 \sqrt{\frac{\log n}{d_{min}}} - \frac{(h(G)-\frac{1}{2})^2}{C_1}\cdot(p_{\mathrm{in}} + p_{\mathrm{out}})  \Bigr] \Biggr).
\]
This completes the proof.
\end{proof}

\subsection{Proof of Theorem 4.1}\label{the:4.1} 
\begin{lemma}\cite{tang2023towards}\label{th3}
    let $n,m$ be the labeling node number and unlabeling number. With some assumptions hold. Suppose that the learning rate $\{\eta_t\}$ satisfies $\eta_t = \frac{2}{\mu(t+t_0)}$ such that $t_0 \geq {\rm max}\{ \frac{2}{\mu}(2P)^{\frac{1}{\alpha}}, 1 \}$. For any $\delta \in (0,1)$, with probability $1-\delta$, 
        \begin{itemize}
        \item[(a).] If $\alpha \in (0, \frac{1}{2})$, we have
        \end{itemize}
        \begin{equation*}\small
        \begin{aligned}
        & \mathcal{L}_{Te}(\mathbf{w}^{(T+1)}) - \mathcal{L}_{Tr}(\mathbf{w}^*) \\
        = & \mathcal{O} \bigg( L_F \frac{{(m+u)}^{\frac{3}{2}}}{mu} \log^{\frac{1}{2}}(T)T^{\frac{1}{2}-\alpha}\log \bigg( \frac{1}{\delta} \bigg) + \frac{1}{T^\alpha} \bigg),
        \end{aligned}
        \end{equation*}
        \begin{itemize}
        \item[(b).] If $\alpha = \frac{1}{2}$, we have
        \end{itemize}
        \begin{equation*}\small
        \begin{aligned}
            & \mathcal{L}_{Te}(\mathbf{w}^{(T+1)}) - \mathcal{L}_{Tr}(\mathbf{w}^*) \\
            = & \mathcal{O} \bigg( L_F \frac{{(m+u)}^{\frac{3}{2}}}{mu} \log(T) \log \bigg( \frac{1}{\delta} \bigg) + \frac{1}{T^\alpha} \bigg).
        \end{aligned}
        \end{equation*}
        \begin{itemize}
        \item[(c).] If $\alpha \in (\frac{1}{2}, 1)$, we have
        \end{itemize}
        \begin{equation*}\small
        \begin{aligned}
            & \mathcal{L}_{Te}(\mathbf{w}^{(T+1)}) - \mathcal{L}_{Tr}(\mathbf{w}^*) \\
            = & \mathcal{O} \bigg( L_F \frac{{(m+u)}^{\frac{3}{2}}}{mu} \log^{\frac{1}{2}}(T) \log (1/\delta) + \frac{1}{T^\alpha} \bigg).
        \end{aligned}
        \end{equation*}
        \begin{itemize}
        \item[(d).] If $\alpha = 1$, we have
        \end{itemize}
        \begin{equation*}\small
        \begin{aligned}
             & \mathcal{L}_{Te}(\mathbf{w}^{(T+1)}) - \mathcal{L}_{Te}(\mathbf{w}^*) \\
             = & \mathcal{O} \bigg( L_F \frac{{(m+u)}^{\frac{3}{2}}}{mu} \log^{\frac{1}{2}}(T) \log (1/\delta) + \frac{\log(T) \log^3 (1/\delta)}{T} \bigg).
        \end{aligned}
        \end{equation*}
\end{lemma}
where  $w$ is weight of the GNN, the training and test error is defined as $\mathcal{L}_{Tr}(\mathbf{w}) \triangleq \frac{1}{m}\sum_{i=1}^{m} \mathcal{L} (\mathbf{w}; Z_i)$ and $\mathcal{L}_{Te}(\mathbf{w}) \triangleq \frac{1}{u}\sum_{i=m+1}^{m+u} \mathcal{L} (\mathbf{w}; Z_i)$ respectively,

\begin{assumption}[Curvature Lower Bound]
\label{assump:curvature_lower_bound}
There exists a constant \( L_F > 0 \) such that for all \( \lambda \in [0,1] \),
\[
(\theta_a - \theta_b)^\top \nabla^2 L(\theta_\lambda) (\theta_a - \theta_b) \ge L_F \|\theta_a - \theta_b\|_2^2.
\]
\end{assumption}

Under this assumption, we have the following result.

\begin{lemma}[Loss Barrier Lower Bound]
\label{thm:loss_barrier_lower_bound}
Under Assumption~\ref{assump:curvature_lower_bound}, the loss barrier satisfies
\[
B(\theta_a,\theta_b) \ge \frac{L_F}{8}\|\theta_a-\theta_b\|_2^2.
\]
\end{lemma}

\begin{proof}
Define the function
\[
\phi(\lambda) := L(\theta_\lambda), \quad \lambda \in [0,1].
\]
Since \( L(\theta) \) is twice differentiable, so is \( \phi(\lambda) \). By Taylor's theorem (or the midpoint error formula) applied at \( \lambda = \frac{1}{2} \), there exists some \( \eta \in (0,1) \) such that
\[
\phi\left(\frac{1}{2}\right) = \frac{1}{2}\Big[\phi(0)+\phi(1)\Big] + \frac{1}{8}\phi''(\eta).
\]
Note that along the interpolation path, the second derivative of \( \phi \) is given by
\[
\phi''(\lambda) = (\theta_a-\theta_b)^\top \nabla^2 L(\theta_\lambda)(\theta_a-\theta_b).
\]
By Assumption~\ref{assump:curvature_lower_bound}, for any \( \lambda \in [0,1] \) we have
\[
\phi''(\lambda) \ge L_F \|\theta_a-\theta_b\|_2^2.
\]
In particular, at \( \lambda = \eta \) it holds that
\[
\phi''(\eta) \ge L_F \|\theta_a-\theta_b\|_2^2.
\]
Thus,
\[
\phi\left(\frac{1}{2}\right) \ge \frac{1}{2}\Big[\phi(0)+\phi(1)\Big] + \frac{L_F}{8}\|\theta_a-\theta_b\|_2^2.
\]
By the definition of the loss barrier,
\[
B(\theta_a,\theta_b) = \max_{\lambda \in [0,1]} \left\{ \phi(\lambda) - \Big[\lambda \phi(1) + (1-\lambda)\phi(0)\Big] \right\} \ge \phi\left(\frac{1}{2}\right) - \frac{1}{2}\Big[\phi(0)+\phi(1)\Big].
\]
Combining the above inequalities yields
\[
B(\theta_a,\theta_b) \ge \frac{L_F}{8}\|\theta_a-\theta_b\|_2^2.
\]
This completes the proof.
\end{proof}
\noindent\textbf{Combine the lemma above, we can achieve the theorem}
\begin{theorem}[Generalization Bound via Loss Barrier]  
\label{thm:generalization-barrier}  
 Let \(\theta^T_a,\theta^T_b\) be the model parameter obtained after \(T\) training iterations under different initialization, with \(m\) labeled and \(n-m\) unlabeled data samples . Then, for any \(\delta \in (0,1)\), with probability at least \(1 - \delta\), the generalization gap satisfies  
\begin{equation}
\Delta_{\text{gen}} \leq O \bigg(  B(\theta_a, \theta_b)\cdot \frac{n^{\frac{3}{2}}}{m(n-m)} \cdot \log(c(T)) T^\rho \log \frac{1}{\delta} \bigg).
\end{equation}
\end{theorem}
\subsection{Proof of Theorical conclusion}
\label{the:final}
\begin{lemma}
(Wasserstein Distance Bounds Performance Gap in GNN Domain Adaptation). Let $P_s(G, Y)$ and $P_t(G, Y)$ be the source and target domain distributions over graphs $G$ and labels $Y$, respectively. Consider a Graph Neural Network (GNN) model $f: G \to Y$ with a loss function $\ell: Y \times Y \to \mathbb{R}^+$. Define the expected loss in each domain as:
\begin{equation}
    \mathbb{E}_{G \sim P_s} [\ell(f(G), Y)] \quad \text{and} \quad \mathbb{E}_{G \sim P_t} [\ell(f(G), Y)].
\end{equation}

Then, the performance gap satisfies the following upper bound:
\begin{equation}
    \left| \mathbb{E}_{G \sim P_t} [\ell(f(G), Y)] - \mathbb{E}_{G \sim P_s} [\ell(f(G), Y)] \right| \leq W_1(\mathcal{L}_s, \mathcal{L}_t) + \lambda,
\end{equation}
where:
\begin{itemize}
    \item $\mathcal{L}_s$ and $\mathcal{L}_t$ denote the loss distributions in the source and target domains, respectively.
    \item $W_1(\mathcal{L}_s, \mathcal{L}_t)$ is the Wasserstein-1 distance:
    \begin{equation}
        W_1(\mathcal{L}_s, \mathcal{L}_t) = \inf_{\gamma \in \Gamma(\mathcal{L}_s, \mathcal{L}_t)} \mathbb{E}_{(\ell_s, \ell_t) \sim \gamma} [|\ell_s - \ell_t|],
    \end{equation}
    where $\Gamma(\mathcal{L}_s, \mathcal{L}_t)$ represents the set of all joint distributions whose marginals are $\mathcal{L}_s$ and $\mathcal{L}_t$.
    \item $\lambda$ is a hypothesis complexity term that depends on the GNN model class $\mathcal{H}$.
\end{itemize}
\end{lemma}

\begin{proof}
We define the performance gap as:
\begin{equation}
    \Delta_{\text{perf}} = \mathbb{E}_{G \sim P_t} [\ell(f(G), Y)] - \mathbb{E}_{G \sim P_s} [\ell(f(G), Y)].
\end{equation}
Applying the triangle inequality:
\begin{equation}
    |\Delta_{\text{perf}}| \leq \sup_{f \in \mathcal{H}} \left| \mathbb{E}_{G \sim P_t} [\ell(f(G), Y)] - \mathbb{E}_{G \sim P_s} [\ell(f(G), Y)] \right|.
\end{equation}

Using the Kantorovich-Rubinstein duality theorem:
\begin{equation}
    W_1(\mathcal{L}_s, \mathcal{L}_t) = \sup_{\|\phi\|_{\text{Lip}} \leq 1} \left| \mathbb{E}_{G \sim P_s} [\phi(\ell_s)] - \mathbb{E}_{G \sim P_t} [\phi(\ell_t)] \right|.
\end{equation}
Choosing $\phi(x) = x$ (which satisfies the Lipschitz constraint), we obtain:
\begin{equation}
    W_1(\mathcal{L}_s, \mathcal{L}_t) \geq \left| \mathbb{E}_{G \sim P_s} [\ell(f(G), Y)] - \mathbb{E}_{G \sim P_t} [\ell(f(G), Y)] \right|.
\end{equation}
Thus,
\begin{equation}
    \left| \mathbb{E}_{G \sim P_t} [\ell(f(G), Y)] - \mathbb{E}_{G \sim P_s} [\ell(f(G), Y)] \right| \leq W_1(\mathcal{L}_s, \mathcal{L}_t).
\end{equation}
Finally, incorporating the hypothesis complexity term $\lambda$ that accounts for model class constraints, we obtain:
\begin{equation}
    \left| \mathbb{E}_{G \sim P_t} [\ell(f(G), Y)] - \mathbb{E}_{G \sim P_s} [\ell(f(G), Y)] \right| \leq W_1(\mathcal{L}_s, \mathcal{L}_t) + \lambda.
\end{equation}
This completes the proof.
\end{proof}
\paragraph{Remark.}  
In fact, this is a general lemma for domain adaptation. Our theorem is a special case of this lemma and follows as a straightforward consequence.
